# Supplementary material for: Generative Models for Fast Calorimeter Simulation.LHCb case
Source: arXiv:1812.01319 source file (2019-04-06)
Supplement: Supplementary file 1 [file appendix.tex]

\section{Appendix}
To define cluster parameters let us consider one calorimeter response produced by one particle. The MC truth information consists of particle's coordinates on the face of the calorimeter, $(x_0, y_0)$, and momentum of the particle on the face of the calorimeter,
 $(p_x, p_y, p_z)$. Depth of the shower maximum ($z_{showerMax}$ is an approximate average depth in Z for energies deposited in different calorimeter layers. 
Then point with coordinates $(x_{showerMax}, y_{showerMax})$, 
where $x_{showerMax} = x_0 + z_{showerMax} \cdot \frac{p_x}{p_z}$, $y_{showerMax} = y_0 + z_{showerMax} \cdot \frac{p_y}{ p_z}$, 
corresponds to the expected center of the cluster in $X, Y$ plane. Particle trajectory line in   $X, Y$ plane is described by the straight line
$\frac{x-x_{showerMax}}{p_x}  = \frac{y-y_{showerMax}}{p_y}$.

Calorimeter response is a set of energies deposited in every cell of the model calorimeter. 

Transverse cluster asymmetry is defined as a difference of energies in calorimeter cells on the left and on the right sides of the trajectory line, divided
by the total energy in all cluster cells.

Longitudinal cluster asymmetry is  defined as a a difference of energies in calorimeter cells on the forward and back sides of the line which
is orthogonal to the trajectory line and intersect it in the point $(x_{showerMax}, y_{showerMax})$, 
divided by the total energy in all cluster cells.

Cluster coordinate is defined as a mean weighted coordinate of the cluster cells: 
$(x_{cluster}, y_{cluster}) = \sum_{cells} (x_{cell}, y_{cell}) \cdot E_{cell}$.

Cluster sparsity for the given threshold is defined as ratio of number of cells with energy above the threshold
to the total number of cells. At very small threshold cluster sparsity represents the fraction of cells with
non-zero energies.
